# Supplementary material for: Augmented Lagrangian Method for Last-Iterate Convergence for Constrained MDPs
Source: arXiv:2605.11694 source file (2026-05-12)
Supplement: Supplementary file 2 [file A6_standard_setting_proofs.tex]

\section{Standard Setting Proofs}
As a warm-up, let's see if we can get last-iterate convergence for NPG or SPMA in the standard RL setting.
\subsection{Last-Iterate Convergence for NPG}
To prove the NPG attains last-iterate convergence, in the following lemma, we first relate it's equivalent update between mirror descent (MD) and follow the regularized leader (FTRL).
\begin{lemma}\label{lemma:npg_md_ftrl_same}
Assuming $\pi_0(\cdot | s)$ is uniform,
the closed form update of 
\begin{equation}
    \pi_{t+1}(\cdot  |s) := \argmax_{\pi(\cdot | s) \in \Delta_A} \bracks*{\dpd{\pi(\cdot | s), q^{\pi_t}(s, \cdot)} - \eta \, D_\phi(\pi(\cdot | s), \pi_t(\cdot | s))}
\end{equation}
or
\begin{equation}
    \bar{\pi}_{t+1}(\cdot  |s) := \argmax_{\pi(\cdot | s) \in \Delta_A} \bracks*{\eta \, \dpd{\pi(\cdot | s), \sum_{j=1}^t q^{\pi_j}(s, \cdot)} - \phi(\pi(\cdot | s))}
\end{equation}
with $\phi(\pi(\cdot | s)) = \sum_{a} \pi(a | s) \, \ln(\pi(a | s))$ results in the the natural policy gradient update
\begin{equation}
    \pi_{t+1}(a | s) = \frac{\pi_t(a | s) \exp(\eta \, q^{\pi_t}(s, a))}{\sum_{a'} \pi_t(a' | s) \, \exp(\eta \, q^{\pi_t}(s, a'))}
\end{equation}
\end{lemma}
\begin{proof}
Showing the first equation results in the NPG update follows from~\citet[Section 4]{xiao2022convergence}. 
To show the second equation also results in the NPG update,
we solve this problem using Lagrange multipliers.  
For a fixed $s \in \cS$, we formulate the following Lagrangian using Lagrangian multipliers $\{\mu_a\}_{a \in \cA}$ and $\lambda \geq 0$,
\begin{equation}
    \cL(\pi_t, \lambda, \mu) := \eta \, \dpd{\pi(\cdot | s), \sum_{j=1}^t q^{\pi_j}(s, \cdot)} - \sum_{a} \pi(a | s) \, \ln(\pi(a | s))  - \sum_{a} \mu_{a} \pi(a | s) - \lambda \parens*{\sum_{a} \pi(a | s) - 1}.
\end{equation}
Solving for a $\pi(\cdot | s) \in \Delta_A$ that satisfies the KKT conditions, we have
\begin{align*}
    \nabla_{\pi(a | s)}\cL(\pi_t, \lambda, \mu) &= \eta \, \sum_{j=1}^t q^{\pi_j}(s, a) - \ln(\pi(a | s)) - 1 - \mu_a - \lambda = 0 \\
    \implies \pi(a | s) &= \exp\parens*{\eta \, \sum_{j=1}^t q^{\pi_j}(s, a) - 1 - \mu_a - \lambda} \\
    &= \frac{\exp\parens*{\eta \, \sum_{j=1}^t q^{\pi_j}(s, a)}}{\exp(1 + \mu_a + \lambda)}
\end{align*}
Let us set
\begin{equation*}
    \mu_a = 0, \quad \forall a \in \cA \quad \text{;} \quad \exp(1 + \lambda) = \parens*{\sum_{a'} \exp\parens*{\eta \, \sum_{j=1}^t q^{\pi_t}(s, a')}}^{-1}
\end{equation*}
to satisfies the KKT conditions and obtain
\begin{equation}
    \pi_t(a | s) = \frac{\exp\parens*{\eta \, \sum_{j=1}^t q^{\pi_j}(s, a)}}{\sum_{a'} \exp\parens*{\eta \, \sum_{j=1}^t q^{\pi_j}(s, a')}}
\end{equation}
Following Assignment 3, Q2, we can use induction to show the above update is equivalent to NPG. Assuming $\pi_1(\cdot | s)$ is uniform.
\end{proof}
\begin{theorem}[Last-iterate convergence of NPG]
If $\pi^*$ is the optimal policy whose value function is equal to $v^*$, the NPG update with $\eta = \frac{\sqrt{2} \, (1 - \gamma) \sqrt{\ln(A)}}{\sqrt{K}}$, $\pi_1$ is uniform initial policy, i.e $\pi_1(\cdot | s) = \frac{1}{A}$ for all $s \in \cS$, satisfies the following sub-optimality bound:
\begin{equation}
    \supnorm{v^* - v^{\pi_K}} \leq \gO\parens*{\frac{1}{K}}
\end{equation}
\end{theorem}
\begin{proof}
\begin{align*}
    v^* - v^{\pi_K} &= v^* - v^{\bar{\pi}_K} + v^{\bar{\pi}_K} - v^{\pi_K} = v^* - v^{\bar{\pi}_K} - [v^{\pi_K} - v^{\bar{\pi}_K}] \tag{Add/Subtract $v^{\bar{\pi}_K}$}  \\
    &= \frac{1}{K} \parens*{1 - \gamma P_{\pi^*}}^{-1} \bracks*{\sum_{t=1}^K \cT_{\pi^*} v^{\pi_t} - \cT_{\pi_t} v^{\pi_t}}
    - \frac{1}{K} \parens*{1 - \gamma P_{\pi_K}}^{-1} \bracks*{\sum_{t=1}^K \cT_{\pi_K} v^{\pi_t} - \cT_{\pi_t} v^{\pi_t}}  \\
    &= \frac{1}{K} \parens*{1 - \gamma P_{\pi^*}}^{-1} \bracks*{\sum_{t=1}^K \cT_{\pi^*} v^{\pi_t} - \cT_{\pi_t} v^{\pi_t}}
    + \frac{1}{K} \parens*{1 - \gamma P_{\pi_K}}^{-1} \bracks*{\sum_{t=1}^K \cT_{\pi_t} v^{\pi_t} - \cT_{\pi_K} v^{\pi_t}} \numberthis \label{eq:npg_sub_opt_gap_to_bound}
\end{align*}
We know how to bound the first term, so let us focus on the second term. For a fixed $s \in \cS$, 
\begin{align*}
\bracks*{\sum_{t=1}^K \cT_{\pi_t} v^{\pi_t} - \cT_{\pi_K} v^{\pi_t}}(s) &= \sum_{t=1}^K \dpd{\pi_t(\cdot | s) - \pi_K(\cdot | s), q^{\pi_t}(s, \cdot)}.
\end{align*}
We will now show the above term is negative. For a fixed iteration $t$,
\begin{align*}
\underbrace{\eta \, \sum_{j=1}^t \dpd{\pi_t(\cdot | s), q^{\pi_j}(\cdot |s)}}_{= \delta_t} &= \eta \, \dpd{\pi_t(\cdot | s) , q^{\pi_t}} + \eta \, \sum_{j=1}^{t-1} \dpd{\pi_t(\cdot | s) \, q^{\pi_j}(s, \cdot)} - \phi(\pi_t) + \phi(\pi_t) \tag{Add/Subtract $\phi(\pi_t)$}\\
&\geq \eta \, \dpd{\pi_t(\cdot | s) \, q^{\pi_t}} + \max_{\pi(\cdot | s) \in \Delta_A} \bracks*{\eta \, \sum_{j=1}^{t-1} \dpd{\pi(\cdot | s) , q^{\pi_j}(s, \cdot)} - \phi(\pi)} + \phi(\pi_t) \tag{According to~\cref{lemma:npg_md_ftrl_same}} \\
&\geq \underbrace{\eta \, \dpd{\pi_t(\cdot | s) \, q^{\pi_t}}}_{:= \Delta_t} + \eta \, \sum_{j=1}^{t-1} \dpd{\pi_{t-1}(\cdot | s) , q^{\pi_j}(s, \cdot)} - \phi(\pi_{t-1}) + \phi(\pi_t) \\
&= \Delta_t  + \delta_{t-1} - \phi(\pi_{t-1}) + \phi(\pi_t) 
\end{align*}
\begin{equation}
    \implies \delta_t \geq \delta_{t-1} + \Delta_t + \phi(\pi_t) - \phi(\pi_{t-1}).
\end{equation}
Recursing from $t=K$ to $1$,
\begin{align*}
    \implies \sum_{t=1}^K \bracks*{\delta_t - \delta_{t-1}} &\geq \sum_{t=1}^K \Delta_t + \sum_{t=1}^K \phi(\pi_t) - \phi(\pi_{t-1}) \\
    \implies \sum_{t=1}^K \delta_K - \underbrace{\delta_{0}}_{= 0} &\geq \sum_{t=1}^K \Delta_t + \phi(\pi_K) - \phi(\pi_0)
\end{align*}
Recall $\phi(\pi) = \sum_a \pi(a | s) \ln(\pi(a | s))$. Assuming we have $\pi_1(\cdot | s) = \frac{1}{A}$, we have $\pi_1(\cdot | s) = \argmin_{\pi(\cdot | s) \in \Delta_A} \phi(\pi)$ and $\phi(\pi_K) - \phi(\pi_1) \geq 0$. 
Hence,
\begin{align*}
    \implies \eta \, \sum_{t=1}^K \dpd{\pi_t(\cdot | s) - \pi_K(\cdot | s), q^{\pi_t}(\cdot |s)} &\leq 0 \\
\implies \bracks*{\sum_{t=1}^K \cT_{\pi_t} v^{\pi_t} - \cT_{\pi_K} v^{\pi_t}}(s) &= \sum_{t=1}^K \dpd{\pi_t(\cdot | s) - \pi_K(\cdot | s), q^{\pi_t}(s, \cdot)} \leq 0.
\end{align*}
Using the above bound with~\cref{eq:npg_sub_opt_gap_to_bound}, for fixed $s \in \cS$,
\begin{align*}
[v^* - v^{\pi_K}](s) &\leq \frac{1}{K} \parens*{1 - \gamma P_{\pi^*}}^{-1} \bracks*{\sum_{t=1}^K \cT_{\pi^*} v^{\pi_t} - \cT_{\pi_t} v^{\pi_t}}(s)
\implies \supnorm{v^* - v^{\pi_K}} \leq \gO\parens*{1/\sqrt{K}} \tag{Using regret bound of NPG}
\end{align*}
\end{proof}
\subsection{Last-Iterate Proof of SPMA} \begin{lemma}\label{lemma:spma_monotonic} For all $t \in [K]$, using the \SPMA update for any $s \in \cS$, \begin{equation*} v^{\pi_{t+1}}(s) \geq v^{\pi_t}(s). \end{equation*} \end{lemma} \begin{proof} According to the Value Difference Lemma, for consecutive policies $\pi_{t+1}$ and $\pi_t$, for any $s \in \cS$ \begin{align*} v^{\pi_{t+1}}(s) - v^{\pi_t}(s) = \E_{s \sim d^{\pi_{t+1}}}\bracks*{\sum_{a} \pi_{t+1}(a | s)\adv^{\pi_t}(s, a)}. \end{align*} It suffices to show $\sum_{a} \pi_{t+1}(a | s)\adv^{\pi_t}(s, a) \geq 0$: \begin{align*} \sum_{a} \pi_{t+1}(a | s)\adv^{\pi_t}(s, a)  &= \sum_{a} \parens*{\pi_{t}(a | s) \, (1 + \eta \adv^{\pi_t}(s, a)} \, \adv^{\pi_t}(s, a) \tag{Using the SPMA update} \\
   &= \sum_{a} \pi_{t}(a | s) \, \adv^{\pi_t}(s, a) + \eta \sum_{a} [\adv^{\pi_t}(s, a)]^2 \\
   &=\sum_{a} \eta \, [\adv^{\pi_t}(s, a)]^2. \tag{$\sum_{a} \pi_t(a | s) \, \adv^{\pi_t}(s, a) = 0$} \\
   &\geq 0.
\end{align*}
\end{proof}
\begin{theorem}
Using the SPMA update in~\cref{eq:spma_gu_update} with
$\etat = \eta =\min\parens*{\frac{\sqrt{\ln(A)} \, (1 - \gamma)}{\sqrt{3 \, U} \, \sqrt{T}}, \frac{1 - \gamma}{2 \, U}}$, $\pi_0(\cdot | s)$ as the uniform initial policy for all $s \in \cS$, and $U=\frac{1}{1 - \gamma}$ satisfies the following sub-optimality bound: 
\begin{equation}
J(\pi^*) - J(\pi_T) \leq \frac{S}{T \, (1 - \gamma)}\parens*{\frac{\sqrt{T} \, \sqrt{3 \, U } (1 + U) \, \sqrt{\ln(A)}}{(1 - \gamma)} + \frac{2 \, U \, \ln(A)}{1 - \gamma}}.
\end{equation}
\end{theorem}
\begin{proof}
To start, we decompose the sub-optimality of the final policy with the mixture policy
\begin{align*}
    J(\pistar) - J(\pi_T) &= J(\pistar) - J(\bar{\pi}_T) + J(\bar{\pi}_T) - J(\pi_T).
\end{align*}
According to~\cref{theorem:gen_utility_pg}, we have
\begin{equation*}
   J(\pistar) - J(\bar{\pi}_K) \leq \frac{S}{T \, (1 - \gamma)}\parens*{\frac{\sqrt{T} \, \sqrt{3 \, U } (1 + U) \, \sqrt{\ln(A)}}{(1 - \gamma)} + \frac{2 \, U \, \ln(A)}{1 - \gamma}}.
\end{equation*}
It suffices to show $J(\bar{\pi}_K) - J(\pi_K) \leq 0$:
\begin{align*}
   J(\bar{\pi}_T) - J(\pi_T)  &= \E_{s \sim \rho} \bracks*{\frac{1}{T} \sum_{j=1}^T V^{\pi_j}(s) - V^{\pi_T}(s)}.
\end{align*}
Using~\cref{lemma:spma_monotonic}, for any $j \in [T]$, $V^{\pi_j}(s) - V^{\pi_T} \leq 0$.
\end{proof}

\subsection{Why these techniques cannot be directly extend for General Utilities}
According to the value difference lemma for General Utilities~\cref{lemma:gu_value_difference}
for any policies $\pi'$ and $\pi$
\begin{equation*}
   G(\pi') - G(\pi) \leq \frac{1}{1 - \gamma} \E_{s \sim d^{\pi'}}\bracks*{[\cT^{\pi'}_{\gupi} V^{\pi}_{\gupi}](s) - V^{\pi}_{\gupi}(s)}.
\end{equation*}
Hence for $\pi' = \pistar$ and $\pi = \pi_K$,
\begin{align*}
G(\pistar) - G(\pi_K) &=  G(\pistar) - \frac{1}{K} \sum_{j=1}^K G(\pi_j) + \frac{1}{K} \sum_{j=1}^K G(\pi_j) - G(\pi_K) \\
&\leq \frac{1}{K \, (1 - \gamma)} \E_{s \sim d^{\pistar}}\bracks*{ \sum_{t=1}^K [\cT^{\pistar}_{\gupit} V^{\pi_t}_{\gupit}](s) - V^{\pi_t}_{\gupit}(s)} - \parens*{G(\pi_K) - \frac{1}{K} \sum_{j=1}^K G(\pi_j)}
\end{align*}
We can apply the General Utility Value Difference to the first term but not the second due ot the one-sided inequality.
