# Supplementary material for: Augmented Lagrangian Method for Last-Iterate Convergence for Constrained MDPs
Source: arXiv:2605.11694 source file (2026-05-12)
Supplement: Supplementary file 3 [file A3_ALM_proofs_copy.tex]

\section{Inexact Augmented Lagrangian Method for Convex Optimization Problems}\label{appendix:convex_proofs}
\todo[inline]{TODO: change indexing from $k$ to $t$. Change notation of some constants. Update reduction in C.2 to use multiple inequality constraints.}

\subsection{Equality Constrained Problems}
To simplify our analysis and align with classical optimization literature, we consider problems in standard form. 
We first consider the constrained problem
\begin{problem}[Equality Constraint Problem]\label{problem:convex_equality}
\begin{align}
\begin{array}{cl}
\displaystyle \min_{x\in \cX} & \displaystyle f(x) \quad \mathrm{subject\ to} \quad Ax=b,\\
\end{array}
\label{eq:objective}
\end{align}
\end{problem}
where $f$ is a convex function, $\cX$ is a closed and bounded set, $A\in \mathbb{R}^{m\times n}$, $b\in\mathbb{R}^{m}$.
Let $x^*$ denote an optimal solution to~\cref{problem:convex_equality}.
The augmented Lagrangian (AL) function of~\cref{problem:convex_equality} is defined as
\begin{align}
\cL_\beta(x,\lambda) := f(x)+\langle \lambda, Ax-b \rangle + \frac{\beta}{2} \|Ax-b\|^2,
\end{align}
where $\lambda\in\mathbb{R}^m$ is the Lagrange multiplier associated with the linear constraint, and $\beta>0$ is the penalty parameter. 
The AL dual of~\cref{problem:convex_equality} is
\begin{equation}
\max_{\lambda\in\mathbb{R}^{m}}\ d(\lambda) \quad \text{;} \quad d(\lambda):=\min_{x\in \cX} \cL_\beta(x,\lambda).
\end{equation}

Given an Lagrange multiplier $\lk$ at iteration $k$, the AL method for solving~\cref{problem:convex_equality} updates the primal and dual variables via
\begin{align}
x(\lk)=\displaystyle\arg\min_{x \in \cX} \cL_\beta(x,\lk) \quad \text{;} \quad \lkk= \lk + \frac{\beta}{2}\left(Ax(\lk)-b\right).
\label{eq:update}
\end{align}
Since computing the primal update can be computationally infeasible, we consider the inexact variant where finding an approximate solution up to a target $\eps_k > 0$ is sufficient (shown in~\cref{alg:cgal}).
\begin{algorithm}[H]
\begin{algorithmic}[1]
    \STATE \textbf{Input}:
    $x_1 \in \cX$ (primal variable) $\lambda_1 \in \R^m$ (dual variable), $\beta > 0$ (constraint penalty), and the non-negative sequence $\braces*{\eps_k}$.
    \FOR{$k = 1, 2, \dots, K$ }
        \STATE Formulate augmented Lagrangian $\cL_\beta(x, \lambda_k) := f(x) + \dpd{\lambda, Ax - b} + \frac{\beta}{2} \, \normsq{Ax - b}$
    \STATE Find the approximate solution $x_{k+1}$ of the AL subproblem such that \[\cL_\beta(x_{k+1}, \lambda_k) - \min_{x \in \cX} \cL_\beta(x, \lambda_k) \leq \eps_k \]
        \STATE $\lambda_{k+1} = \lambda_k + \frac{\beta}{2} \, (Ax_{k+1} - b)$
        \ENDFOR
    \STATE Return $x_{K+1}$
\end{algorithmic}
\caption{Inexact Augmented Lagrangian Method for Equality Constraints (\cref{problem:convex_equality})}
\label{alg:cgal}
\end{algorithm}
The following notation and relations will be helpful in the proofs:
\begin{align}
x(\lk):=&\arg\min_{x \in \cX} \cL_\beta(x, \lk),~k=1,2,\ldots,\label{xlambda}\\
\nabla d(\lk):=&Ax(\lk)-b,~k=1,2,\ldots,\nonumber\\
\bar d(\lk):=& \cL_{\beta}(\xkk,\lk),~k=1,2,\ldots,\label{bard}\\
\nabla \bar d(\lk):=&A\xkk-b,~k=1,2,\ldots,\label{bardgradient}
\end{align}

As stated in~\cref{alg:cgal}, at iteration $k$, we ensure that the following error condition is satisfied 
\begin{align}
\cL_\beta(\xkk, \lk) - \cL_\beta(x(\lk), \lk) = \bar{d}(\lk)- d(\lk) \leq \epsk.
\label{eq:error-metric}    
\end{align}
\begin{lemma}
In~\cref{alg:cgal}, for all iterations $k \geq 1$,
\begin{align}
\normsq{\nabla d(\lk)-\nabla\bar d(\lk)} \leq \frac{2 \epsk}{\beta}.
\end{align}
\label{lemma:diff-grad}    
\end{lemma}
\begin{proof}
\begin{align}
\normsq{\nabla d(\lk)-\nabla\bar d(\lk)} &= \normsq{A x(\lk) - b - (A \xkk - b)} = \normsq{A x(\lk) - A \xkk}
\label{eq:diff-grad-1}
\end{align}
Define 
\begin{align*}
u^* = A x(\lk) \quad \text{;} \quad \hat u &= A \xkk \quad \text{;} \quad h(u) = \langle \lk,\,u - b\rangle + \frac{\beta}{2} \normsq{u - b} \\
\implies \cL_\beta(x, \lk) & = f(x) + h(Ax)
\end{align*}
Since $h$ is $\beta$-strongly convex in $u$, we have
\begin{align*}
h(\hat u) \;\ge\; h(u^*) +\langle\nabla h(u^*),\,\hat u - u^*\rangle +\frac{\beta}{2} \normsq{\hat u - u^*}.    
\end{align*}
By convexity of $f$, for any $x, y$
\[
f(y)\;\ge\;f(x)+\langle\nabla f(x),\, y - x \rangle.
\]
And the first‐order optimality condition at $x(\lk)$ gives, for all $x \in \cX$, 
\begin{align}
& \langle\nabla \cL_\beta(x(\lk), \lk),\, x - x(\lk) \rangle \geq 0 \implies \langle\nabla f(x(\lk)) + A^T\nabla h(u^*),\,x - x(\lk)\rangle \geq 0 \nonumber \\
\implies & \langle\nabla \cL_\beta(x(\lk), \lk),\, \xkk - x(\lk) \rangle \geq 0 \implies \langle\nabla f(x(\lk)) + A^T\nabla h(u^*),\, \xkk - x(\lk)\rangle \geq 0 \tag{Setting $x = \xkk$} \\
\intertext{Using the definition of $u^*$ and $\hat{u}$}
\implies & \langle\nabla f(x(\lk)),\, \xkk - x(\lk)\rangle + \langle\nabla h(u^*),\, \hat{u} - u^*\rangle \geq 0 \label{eq:opt-condition}
\end{align}

\begin{align*}
\cL_\beta(\xkk, \lk)-\cL_\beta(x(\lk), \lk) &= \left[f(\xkk)-f(x(\lk))\right] + \left[h(\hat u)-h(u^*)\right]\\
& \geq \langle\nabla f(x(\lk)),\, \xkk - x(\lk)\rangle + \left[\langle\nabla h(u^*),\,\hat u - u^*\rangle + \frac{\beta}{2} \normsq{\hat u - u^*} \right] \tag{By convexity of $f$ and strong-convexity of $h$} \\
&\ge \underbrace{\langle\nabla f(x(\lk)),\,\xkk - x(\lk)\rangle +\langle\nabla h(u^*),\,\hat u - u^*\rangle}_{\geq 0 \text{ from~\cref{eq:opt-condition}}}
+ \frac{\beta}{2} \normsq{\hat{u} - u^*} \\
&\geq \frac{\beta}{2} \normsq{A\xkk - A x(\lk)} \tag{By definition of $u^*$ and $\hat{u}$}
\end{align*}
Hence, since $\cL_\beta(\xkk, \lk)-\cL_\beta(x(\lk), \lk) \leq \epsk$, we conclude
\begin{align*}
\normsq{A\xkk - A x(\lk)} \leq \frac{2\epsk}{\beta}.    
\end{align*}
Combining with~\cref{eq:diff-grad-1} finishes the proof. 
\end{proof}


\begin{lemma}
In~\cref{alg:cgal}, for all $k \geq 1$, the following two inequalities hold:
\begin{align}
  d(\lambda) \leq \bar d(\mu) + \left\langle\nabla\bar d(\mu),\lambda-\mu\right\rangle,~\forall~\lambda,\mu,
  \label{eq:d-error-ub}
\end{align}
and
\begin{align}
d(\lkk)\geq\bar d(\lk)+\frac{\beta}{4} \left\|\nabla \bar d(\lk)\right\|^2 - 2 \, \epsk.
\label{eq:d-error-lb}
\end{align}
\label{lemma:d-error}
\end{lemma}
\begin{proof} 
We first show \cref{eq:d-error-ub}. By the definitions of $d(\lambda)$ and $\cL_\beta(x, \lambda)$, we have
\begin{align}
d(\lambda)=\min_{x\in \cX}\left\{\cL_\beta(x,\lambda)\right\}\leq \cL_\beta(x_{\mu},\lambda)=\cL_\beta(x_{\mu},\mu) + \langle\lambda-\mu,Ax_{\mu}-b\rangle, \tag{By definition of $\LCal_\beta(x, \lambda)$ and $\LCal_\beta(x, \mu)$}
\end{align}
where $x_{\mu}$ is defined such that $\bar d(\mu)=\cL_\beta(x_{\mu},\mu)$. This, together with the definition of $\nabla \bar d(\mu) = A x_\mu - b$ yields \cref{eq:d-error-ub}.

\vspace{2ex}

We now prove \cref{eq:d-error-lb}. According to~\cref{lemma:alm_dual_smooth}, $d$ is $\frac{1}{\beta}$-smooth,
\begin{align}
   d(\lkk) &\geq d(\lk) + \langle \nabla  d(\lk), \lkk - \lk \rangle - \frac{1}{2 \, \beta} \, \normsq{\lkk - \lk} \\
   &= d(\lk) + \langle \nabla  d(\lk), \frac{\beta}{2} \, \nabla \bar d(\lk) \rangle - \frac{\beta}{8} \, \normsq{\nabla \bar d(\lk)} \tag{Using the dual update $\lkk = \lk + \frac{\beta}{2} \, \nabla \bar d(\lk)$} \\
   &= \bar d(\lk) + \underbrace{d(\lk) - \bar d(\lk)}_{\geq -\eps_k \text{ from~\cref{eq:error-metric}}} + \langle \nabla  d(\lk), \frac{\beta}{2} \, \nabla \bar d(\lk) \rangle - \frac{\beta}{8} \, \normsq{\nabla \bar d(\lk)} \tag{Add/Subtract $\bar{d}(\lk)$} \\
   &\geq \bar d(\lk) - \eps_k + \langle \nabla  d(\lk) + \nabla \bar d(\lk) - \nabla \bar d(\lk), \frac{\beta}{2} \, \nabla \bar d(\lk) \rangle - \frac{\beta}{8} \, \normsq{\nabla \bar d(\lk)} \tag{Add/Subtract $\langle \nabla \bar{d}(\lk), \nabla \bar{d}(\lk) \rangle$} \\
   &= \bar d(\lk) - \eps_k  + \frac{3\,\beta}{8} \, \normsq{\nabla \bar d(\lk)} - \left[\langle - \frac{\beta}{2} \, \nabla \bar d(\lk), \nabla  d(\lk) - \nabla \bar d(\lk) \rangle \right] \\
   &\geq \bar d(\lk) - \eps_k  + \frac{3 \, \beta}{8} \, \normsq{\nabla \bar d(\lk)} - \frac{\beta}{8} \, \normsq{\nabla \bar d(\lk)} - \frac{\beta}{2} \, \normsq{\nabla  d(\lk) - \nabla \bar d(\lk)}   \tag{Using Young's Inequality, $\langle a, b \rangle \leq \frac{\normsq{a}}{2\,\beta}  + \frac{\beta \, \normsq{b}}{2}$} \\
\implies d(\lkk) &\geq \bar d(\lk) - 2 \, \eps_k  + \frac{\beta}{4} \, \normsq{\nabla \bar d(\lk)}\tag{Using~\cref{lemma:diff-grad}}
\end{align}
\end{proof}


\begin{lemma}
For all $k \geq 1$, 
\begin{align}
\norm{\lk - \lstar} \leq \sqrt{\normsq{\lambda_1- \lstar} + 2 \, \beta \, \sum_{i = 1}^{k-1} \epsilon_i }    
\end{align}
\label{lemma:bounded-dual-iterates}    
\end{lemma}
\begin{proof}
\begin{align*}
\normsq{\lkk - \lstar} &= \normsq{\lk - \frac{\beta}{2} \nabla \bar{d}(\lk) - \lstar} = \normsq{\lk - \lstar} + \beta \langle \nabla \bar{d}(\lk), \lk - \lstar \rangle + \frac{\beta^2}{4} \normsq{\nabla \bar{d}(\lk)} \tag{Using the dual update $\lkk = \lk + \frac{\beta}{2} \, \nabla \bar d(\lk)$}\\
& \leq \normsq{\lk - \lstar} + \beta \, [\bar{d}(\lk)- d(\lstar)] + \frac{\beta^2}{4} \normsq{\nabla \bar{d}(\lk)} \tag{Using \cref{eq:d-error-ub} in~\cref{lemma:d-error} with $\lambda = \lambda^*$ and $\mu = \lk$} \\
& = \normsq{\lk - \lstar} + \underbrace{\beta \, [d(\lkk)- d(\lstar)]}_{\leq 0 \text{ since $\lambda^* := \argmax d(\lambda)$}} + \beta \, [\bar{d}(\lk) - d(\lkk)] + \frac{\beta^2}{4} \, \normsq{\nabla \bar{d}(\lk)} \tag{Add/Subtract $d(\lkk)$} \\
& \leq \normsq{\lk - \lstar} + \beta \, [\bar{d}(\lk) - d(\lkk)] + \beta [d(\lkk) - \bar d(\lk) +  2 \, \eps_k] \tag{Using~\cref{eq:d-error-lb} in~\cref{lemma:d-error} to simplify the last term} \\
& \leq  \normsq{\lk - \lstar} + 2 \, \beta \, \epsk %
\intertext{Hence, by recursing, for all $k \geq 1$,}
\implies \normsq{\lk - \lstar} & \leq \normsq{\lambda_1- \lstar} + 2 \, \beta \, \sum_{i = 1}^{k-1} \epsilon_i 
\end{align*}    
Using that $\sqrt{a+b} \leq \sqrt{a} + \sqrt{b}$ completes the proof. 
\end{proof}



\begin{theorem}\label{thm:convex_linear_equality_constraints_alm_rate}
If $\epsk = \frac{\sigma}{k^{2}}$ with some constant $\sigma>0$ and $\lambda_1 = 0$,~\cref{alg:cgal}  achieves the following convergence: for all $k \geq 1$,
\begin{align}
d(\lambda^*) - d(\lk) & \leq \frac{C}{k} \\ 
\norm{Ax_{k+1}-b}  &\leq \frac{2}{\sqrt{\beta}} \left(\frac{\sqrt{C}}{\sqrt{k}} + \frac{\sqrt{2 \, \sigma}}{k}\right)  \label{eq:cons_iter_bound} \\ 
f(x_{k+1}) - f(x^*)  &\leq \frac{2(D + \norm{\lambda^*})}{\sqrt{\beta}} \left(\frac{\sqrt{C}}{\sqrt{k}} + \frac{\sqrt{2 \, \sigma}}{k}\right) + \frac{\sigma}{k^2} \label{eq:primal_iter_bound}\,,
\end{align}
where $B := \norm{\lambda^*} + \sqrt{\sigma} \, \frac{\beta \, \pi^2}{3}$, $\theta := \frac{\beta}{2 B^2}$, $\omega := 3$, $C := \frac{4}{\theta}\left(1+\sqrt{2\,\omega\sigma\theta(\omega\sigma\theta+1)}\right) + 4\max\left\{\delta_1,\frac{4}{\theta}\right\}$ and $D := \sqrt{\normsq{\lambda_1- \lstar} + 2 \, \beta \, \sum_{i = 1}^{k-1} \epsilon_i }$.
\label{thm:convergence-rate}   
\end{theorem}
\begin{proof}
Using~\cref{eq:d-error-lb} in~\cref{lemma:d-error}, 
\begin{align*}
d(\lkk) &\geq \bar d(\lk) + \frac{\beta}{4} \, \normsq{\nabla \bar d(\lk)} - 2 \eps_k  \\
\intertext{Since by definition, $\bar{d}(\lk) \geq d(\lk)$,}
& \geq d(\lk) + \frac{\beta}{4} \normsq{\nabla \bar{d}(\lk)} - 2 \epsk \\
\intertext{Since $\normsq{\nabla d(\lk)} = \normsq{\nabla d(\lk) - \nabla \bar{d}(\lk) + \nabla \bar{d}(\lk)} \leq 2 \, \normsq{\nabla d(\lk) - \nabla\bar{d}(\lk)} + 2 \, \normsq{\nabla\bar{d}(\lk)}$. Hence, $\normsq{\nabla\bar{d}(\lk)} \geq \frac{1}{2} \normsq{\nabla d(\lk)} - \normsq{\nabla d(\lk) - \nabla \bar{d}(\lk)}$. Hence,}
& \geq d(\lk)+ \frac{\beta}{8} \normsq{\nabla d(\lk)} - \frac{\beta}{4} \, \normsq{\nabla d(\lk) - \nabla \bar{d}(\lk)} - 2 \epsk \\
\implies d(\lambda^*) - d(\lkk) & \leq d(\lambda^*) - d(\lk) - \frac{\beta}{8} \, \normsq{\nabla d(\lk)} + \frac{\beta}{4} \, \normsq{\nabla d(\lk) - \nabla \bar{d}(\lk)} + 2\epsk \\
& \leq \underbrace{d(\lambda^*) - d(\lk)}_{:= \delta_k} - \frac{\beta}{8} \, \normsq{\nabla d(\lk)} + 3 \epsk \tag{Using~\cref{lemma:diff-grad}} \\
\implies \delta_{k+1} & \leq \delta_k - \frac{\beta}{8} \, \normsq{\nabla d(\lk)} + 3 \epsk
\end{align*}
Since $d(\lambda)$ is concave in $\lambda$, 
\begin{align*}
d(\lstar) - d(\lk) & \leq \langle \nabla d(\lk), \lstar - \lk \rangle \leq \norm{\nabla d(\lk)} \, \norm{\lk - \lstar} \tag{Cauchy Schwarz} \\
& \leq \norm{\nabla d(\lk)} \, \sqrt{\normsq{\lambda_1- \lstar} + 2 \, \beta \, \sum_{i = 1}^{k-1} \epsilon_i } \tag{Using~\cref{lemma:bounded-dual-iterates}} \\
& \leq \norm{\nabla d(\lk)} \, \left[\norm{\lambda^*} + \sqrt{2 \, \sigma \, \beta \, \sum_{i = 0}^{k-1} \frac{1}{i^2}} \right] \tag{Using that $\lambda_1 = 0$,  $\sqrt{a+b} \leq \sqrt{a} + \sqrt{b}$ and $\epsk = \frac{\sigma}{k^2}$} \\
& \leq \norm{\nabla d(\lk)} \, \underbrace{\left[\norm{\lambda^*} + \sqrt{\frac{\sigma \, \beta \, \pi^2}{3}} \right]}_{:= B} \tag{$\sum_{i = 0}^{k-1} \frac{1}{i^2} \leq \sum_{i = 0}^{\infty} \frac{1}{i^2} = \frac{\pi^2}{6}$} \\
\implies \norm{\nabla d(\lk)} & \geq \frac{d(\lstar) - d(\lk)}{B} = \frac{\delta_k}{B}
\end{align*}
Combining the above relations, 
\begin{align*}
\delta_{k+1} & \leq \delta_k - \frac{\beta}{8 \, B^2} \, \delta_k^2 + 3 \epsk     
\end{align*}
Using~\cref{lemma:delta-bound}, we can now conclude that for $\eps_k = \frac{\sigma}{k^2}$, $\theta = \frac{\beta}{8 B^2}$ and $\omega = 3$, if $C := \frac{4}{\theta}\left(1+\sqrt{2\,\omega\sigma\theta(\omega\sigma\theta+1)}\right) + 4\max\left\{\delta_1,\frac{4}{\theta}\right\}$, for all $k \geq 1$,
\begin{align*}
\delta_k \leq \frac{C}{k}    
\end{align*}
Now we will use the above result to bound the constraint violation and sub-optimality. Using the above relations, we know that, 
\begin{align*}
d(\lkk) & \geq d(\lk)+ \frac{\beta}{4} \normsq{\nabla \bar{d}(\lk)} - 2 \epsk \\
\end{align*}
Since $\nabla \bar{d}(\lk) = A \xkk - b$, 
\begin{align*}
\left\|Ax_{k+1}-b\right\|^2 \leq  \frac{4}{{\beta}}\left(d(\lambda_{k+1})- d(\lambda_k)+ 2 \, \epsk \right) \leq & \ \frac{4}{{\beta}}\left(d(\lambda^*)-d(\lk)+ 2 \, \epsk\right) = \frac{4}{{\beta}}\left(\delta_k+ 2 \, \epsk \right) \leq \frac{4}{\beta} \left(\frac{C}{k} + \frac{2 \, \sigma}{k^2}\right) \\
\implies \norm{Ax_{k+1}-b} & \leq \frac{2}{\sqrt{\beta}} \left(\frac{\sqrt{C}}{\sqrt{k}} + \frac{\sqrt{2 \, \sigma}}{k}\right) 
\end{align*}
We will now bound the sub-optimality. 
\begin{align*}
\cL_\beta(\xkk,\lk) &= \cL_\beta(\xkk,\lk) - \cL_\beta(x(\lk),\lk) + \cL_\beta(x(\lk),\lk) \leq \cL_\beta(x(\lk),\lk) + \epsk \\
& = d(\lk) + \epsk \tag{By definition of $d(\lk)$} \\
& \leq d(\lambda^*) + \epsk \tag{Since $\lambda^* = \argmax d(\lambda)$} \\
& = f(x^*) + \epsk \tag{Strong duality}
\end{align*}
\begin{align*}
\implies f(\xkk) + \langle \lk, A \xkk - b \rangle + \frac{\beta}{2} \normsq{A \xkk - b} & \leq f(x^*) + \epsk \tag{By definition of $\cL_\beta(\xkk, \lk)$} \\
\implies f(\xkk) & \leq f(x^*) + \norm{\lk} \, \norm{A \xkk - b} + \epsk \tag{Cauchy Schwarz} \\
& \leq f(x^*) + (\norm{\lk - \lambda^*} + \norm{\lambda^*}) \, \norm{A \xkk - b} + \epsk \tag{Triangle inequality} \\
& \leq f(x^*) + (D + \norm{\lambda^*}) \, \norm{A \xkk - b} + \epsk \tag{Using~\cref{lemma:bounded-dual-iterates}} \\
\implies f(\xkk) - f(x^*) & \leq \frac{2(D + \norm{\lambda^*})}{\sqrt{\beta}} \left(\frac{\sqrt{C}}{\sqrt{k}} + \frac{\sqrt{2 \sigma}}{k}\right) + \frac{\sigma}{k^2} \tag{Using the bound on the constraint violation}
\end{align*}
\end{proof}


\todo[inline]{The following corollary is incorrect, need a new version of~\cref{lemma:delta-bound} since it depends on $\eps_k = \frac{1}{k^2}$.}
\begin{corollary}\label{cor:thm:convergence-rate-log-eqaulity}
If $\epsk = \frac{\sigma}{k \, \ln(K)}$ with some constant $\sigma>0$ and $\lambda_1 = 0$,~\cref{alg:cgal}  achieves the following convergence for all $k \in [1, K]$: 
\end{corollary}



\subsection{Reduction from Equality to Inequality Constrained Problems}
Next, we extended the results of~\cref{thm:convergence-rate} to handle inequality constraints without any additional analysis.
We now consider the following constraint problem where for simplicity we consider a single inequality constraint with $a \in \R^n$
\begin{problem}[Inequality Constraint Problem]\label{problem:convex_inequality}
\begin{align}
\begin{array}{cl}
\displaystyle \min_{x\in \cX} & \displaystyle f(x) \quad \mathrm{subject\ to} \quad \dpd{a, x} \leq b,
\end{array}
\label{eq:objective_inequality}
\end{align}
\end{problem}
The AL for~\cref{problem:convex_inequality} is defined as
\begin{equation}\label{eq:al_convex_inequality}
   \cL^\dagger_\beta(x, \lambda) := f(x) + \frac{\beta}{2} \, \parens*{\bracks*{\max\parens*{\dpd{a, x} - b + \frac{\lambda}{\beta}, 0}}^2  - \frac{\lambda^2}{\beta^2}} 
\end{equation}
and the inexact AL method for~\cref{problem:convex_inequality} is presented in~\cref{alg:inexact_alm_convex_ineq_constraints}.
\begin{algorithm}[H]
\begin{algorithmic}[1]
    \STATE \textbf{Input}:
    $x_1 \in \cX$ (primal variable) $\lambda_1 \in \R$ (dual variable), $\beta > 0$ (constraint penalty), and the non-negative sequence $\braces*{\eps_k}$.
    \FOR{$k = 1, 2, \dots, K$ }
    \STATE Formulate augmented Lagrangian $\cL^\dagger_\beta(x, \lambda_k) := f(x) + \frac{\beta}{2} \, \parens*{\bracks*{\max\parens*{\dpd{a, x} - b + \frac{\lambda_k}{\beta}, 0}}^2  - \frac{\lambda_k^2}{\beta^2}}$
    \STATE Find the approximate solution $x_{k+1}$ of the AL subproblem such that \[\cL^\dagger_\beta(x_{k+1}, \lambda_k) - \min_{x \in \cX} \cL^\dagger_\beta(x, \lambda_k) \leq \eps_k \]
        \STATE $\lambda_{k+1} = \lambda_k + \frac{\beta}{2} \, (Ax_{k+1} - b)$
        \ENDFOR
    \STATE Return $x_{K+1}$
\end{algorithmic}
\caption{Inexact Augmented Lagrangian Method for Inequality Constrains (\cref{problem:convex_inequality})}
\label{alg:inexact_alm_convex_ineq_constraints}
\end{algorithm}

Before proceduing with the reduction, we make the following remarks

1. Any Inequality constraint problem is equivlaent to an equation constraint problem by add slack variables.

2 Finding an approximate solution to the Inequality constraint AL subproblem
yields a valid solutin for the equality constraint with slack variable0






\begin{lemma}\label{lemmma:alm_inequality_constraint}
If $\eps_k = \frac{\sigma}{k^2}$ with some constant $\sigma > 0$ and $\lambda_1 = 0$,~\cref{alg:inexact_alm_convex_ineq_constraints} achieves the following convergence: for all $k \geq 1$,
\begin{align*}
   \max(\dpd{a, \xkk} -b, 0)  &\leq  \frac{2}{\sqrt{\beta}} \left(\frac{\sqrt{C}}{\sqrt{k}} + \frac{\sqrt{2 \, \sigma}}{k}\right) \\
   f(\xkk) - f(x^*) &\leq \frac{2(D + \norm{\lambda^*})}{\sqrt{\beta}} \left(\frac{\sqrt{C}}{\sqrt{k}} + \frac{\sqrt{2 \, \sigma}}{k}\right),
\end{align*}
where $B := \norm{\lambda^*} + \sqrt{\sigma} \, \frac{\beta \, \pi^2}{3}$, $\theta := \frac{\beta}{2 B^2}$, $\omega := 3$, $C := \frac{4}{\theta}\left(1+\sqrt{2\,\omega\sigma\theta(\omega\sigma\theta+1)}\right) + 4\max\left\{\delta_1,\frac{4}{\theta}\right\}$ and $D := \sqrt{\normsq{\lambda_1- \lstar} + 2 \, \beta \, \sum_{i = 1}^{k-1} \epsilon_i }$.
\end{lemma}
\begin{proof}
To extend the results of~\cref{thm:convergence-rate}, we first show finding an $\eps$-close solution to~\cref{eq:al_convex_inequality} yields a solution to an equivalent AL subproblem with equality constraints.
We first add slack variables $s$ to~\cref{problem:convex_inequality} in order to convert the inequality constraints to enforce equality constrains
\begin{problem}[Equality Constraint Problem with Slack Variables]\label{problem:convex_equality_slack}
\begin{align}
\begin{array}{cl}
\displaystyle \min_{x\in \cX} & \displaystyle f(x) \quad \mathrm{subject\ to} \quad \dpd{a, x} + s^2 = b.
\end{array}
\label{eq:objective_equality_slack}
\end{align}
\end{problem}
The AL of~\cref{problem:convex_equality_slack} is defined as
\begin{equation}\label{eq:al_slack}
    \tilde{\cL}_\beta(x, s, \lambda) := f(x) + \lambda \, [\dpd{a, x} - b + s^2] + \frac{\beta}{2} \, [\dpd{a, x} - b + s^2]^2.
\end{equation}
In each iteration $k$,~\cref{alg:inexact_alm_convex_ineq_constraints} guarantees a point $\xkk$ such that
\begin{equation*}
\cL^\dagger_\beta(x_{k+1}, \lambda_k) - \min_{x \in \cX} \cL^\dagger_\beta(x, \lambda_k) \leq \eps_k 
\end{equation*}
According to~\cref{lemma:aug_lag_subproblem_same}, the pair $(\xkk, s_{k+1})$ where $s_{k+1} = \max\parens*{0, - \frac{\lambda}{\beta} - \dpd{a, \xkk} + b}$ satisfies 
\begin{align}
    \tilde{\cL}_\beta(\xkk, s_{k+1}, \lambda) - \min_{x \in \cX, s \in \R}\tilde{\cL}_\beta(x, s, \lambda_k) \leq \eps.
\end{align}
Next, we apply a transformation to~\cref{problem:convex_equality_slack} to convert it into standard form.
Define
\begin{align*}
   \mathbf{A} := \begin{bmatrix} a & 0\\ 0 & 1 \end{bmatrix} \quad \text{;} \quad \mathbf{x} := \begin{bmatrix} x \\ s^2 \end{bmatrix} \quad \text{;} \quad  \mathbf{f}(\mathbf{x}) := f(x) \quad \text{;} \quad \cD := \cX \times \R.
\end{align*}
Hence,~\cref{problem:convex_equality_slack} is equivalent to
\begin{align}\label{eq:objective_equality_trans}
\begin{array}{cl}
\min_{\mathbf{x} \in \cD} \displaystyle \mathbf{f}(\mathbf{x}) \quad \text{subject to} \quad \mathbf{A} \mathbf{x} = b,
\end{array}
\end{align}
and with a slight abuse of notation let $\tilde{\cL}_\beta(\mathbf{x}, \lambda) = \tilde{\cL}_\beta(x, s, \lambda)$.
Next we use the results of~\cref{thm:convergence-rate} to bound the constraint violation and sub-optimality.
To bound the constraint violations, at iteration $k \geq 1$,
\begin{align*}
    \max(\dpd{a, \xkk} -b, 0) &\leq \dpd{a, \xkk} -b \\
    &= \dpd{a, \xkk} -b + [s_{k+1}]^2 \tag{$[s_{k+1}]^2 \geq 0$} \\
    &\leq \abs{\dpd{a, \xkk} -b + [s_{k+1}]^2} \\
    &= \normsq{ \mathbf{A} \mathbf{x}_{k+1} - b}  \\
    \implies \max(\dpd{a, \xkk} -b, 0) &\leq \frac{2}{\sqrt{\beta}} \left(\frac{\sqrt{C}}{\sqrt{k}} + \frac{\sqrt{2 \, \sigma}}{k}\right) \tag{Using~\cref{eq:cons_iter_bound} of~\cref{thm:convergence-rate}}
\end{align*}
Additionally, the sub-optimality can be bounded as
\begin{align*}
f(\xkk) - f(x^*) &\leq \mathbf{f}(\mathbf{x}_{k+1}) - \mathbf{f}(\mathbf{x}^*) \tag{The set of feasible points of~\cref{problem:convex_equality_slack} is a subset of~\cref{problem:convex_inequality}} \\
&\leq \frac{2(D + \norm{\lambda^*})}{\sqrt{\beta}} \left(\frac{\sqrt{C}}{\sqrt{k}} + \frac{\sqrt{2 \, \sigma}}{k}\right). \tag{Using~\cref{eq:primal_iter_bonud} of~\cref{thm:convergence-rate}}
\end{align*}
\end{proof}

\todo[inline]{The following corollary is incorrect, need a new version of~\cref{lemma:delta-bound} since it depends on $\eps_k = \frac{1}{k^2}$.}
\begin{corollary}\label{cor:alm_inequality_constraint_log_fixed_K}
If $\eps_k = \frac{\sigma}{k \, \log(K)}$ with some constant $\sigma > 0$ and $\lambda_1 = 0$,~\cref{alg:inexact_alm_convex_ineq_constraints} achieves the following convergence: for fixed iteration $K \geq 1$,
\end{corollary}



\subsection{Additional Lemmas}
\begin{lemma}
For $k \geq 1$, if $\delta_k \geq 0$, a constant $\theta \geq 0$ and $\epsk = \frac{\sigma}{k^{2}}$, if 
\begin{align*}
\delta_{k+1} & \leq \delta_k - \theta \, \delta_k^2 + \omega \epsk \,,    
\end{align*}
then, for all $k \geq 1$, 
\begin{align}
\delta_{k} \leq \frac{C}{k} \text{ where } C := \frac{4}{\theta}\left(1+\sqrt{2\,\omega\sigma\theta(\omega\sigma\theta+1)}\right)
+ 4\max\left\{\delta_1,\frac{4}{\theta}\right\}.
\label{deltaeta-global}
\end{align}
\label{lemma:delta-bound}
\end{lemma}
\begin{proof}
We will follow the proof in~\citet[Theorem 4.3]{liu2019nonergodic} and do the proof by induction. Clearly, the inequality \eqref{deltaeta-global} holds for $k=1$. Next, we assume that \eqref{deltaeta-global} holds for some $k\geq 1$, and show it is also true for $k+1$. We use the contrapositive argument. Assume that \eqref{deltaeta-global} does not hold for $k+1$, i.e.,
\begin{align}
\delta_{k+1} > \frac{C}{k+1},
\label{eq:nothold}
\end{align}
In this case, we define $z^* :=\frac{C}{4}-\frac{1}{\theta}>0$ and will subsequently prove that
\begin{align*}
&\frac{\theta}{2} \left(\delta_{k+1}-\frac{z^*}{(k+1)}\right)^2 + \left(\delta_{k+1}-\frac{z^*}{(k+1)}\right) \leq \left(\delta_{k}-\frac{z^*}{k}\right) \\ 
&\Leftrightarrow P(z^*)  := \frac{\theta}{2} \left(\delta_{k+1}-\frac{z^*}{(k+1)}\right)^2 + \left(\delta_{k+1}-\frac{z^*}{(k+1)}\right)- \left(\delta_{k}-\frac{z^*}{k}\right)\leq0.
\end{align*}
If the $P(z^*) \leq 0$, then, it follows from Lemma \ref{prop:1} that
\begin{align}
\label{eq:final}
\delta_{k+1}-\frac{z^*}{(k+1)} \leq \frac{\max\left\{\delta_1,\frac{4}{\theta}\right\}}{k+1} \implies \delta_{k+1}\leq \frac{z^* + \max\left\{\delta_1,\frac{4}{\theta}\right\}}{(k+1)} < \frac{C}{(k+1)}.
\end{align}
Clearly, \eqref{eq:final} contradicts \eqref{eq:nothold}, which implies that \eqref{deltaeta-global} is true and completes the inductive step. 

Now, we will prove that if~\cref{eq:nothold} holds, then, $P(z^*) \leq 0$. For this, we consider the following quadratic function $Q(z)$ with respect to $z:$
\begin{eqnarray*}\label{eq:quad}
Q(z) = \frac{\theta}{2}z^2 - \left(\frac{\theta C}{4}-1\right)z + \omega\left(\omega \theta \sigma +1\right)\sigma.
\end{eqnarray*}
It can be verified that for the minimizer of $Q(z)$ is $z^*$, and that for $C$ defined in the theorem statement, 
\begin{equation}\label{Qz*}
    Q(z^*)\leq 0.
\end{equation}
Moreover, for any $k\geq 1$, we know that, 
\begin{align*}
\delta_{k+1} & \leq \delta_k - \theta \, \delta_k^2 + \omega \epsk \implies \delta_{k+1} \leq \delta_k + \omega  \epsk \Longrightarrow 
\frac{1}{2}\delta_{k+1}^2 \leq \delta_k^2 + \omega^2 \epsk^2\Longrightarrow-\delta_k^2 \leq -\frac{1}{2}\delta_{k+1}^2 + \omega^2 \sigma\epsk. \tag{Since $\epsk \leq \frac{\sigma}{k^2}$}    
\end{align*}



Combining the last inequality in the above with the condition in the statement yields
\begin{align}
\label{eq:ineqnoise2}
\delta_{k+1} & \leq \delta_k - \theta \, \delta_k^2 + \omega \epsk \implies \delta_{k+1} \leq \delta_k + \theta \, \left[-\frac{1}{2}\delta_{k+1}^2 + \omega^2 \sigma\epsk \right] + \omega \epsk \\
\implies \frac{\theta}{2}\delta_{k+1}^2 + \delta_{k+1} & \leq \delta_k  + \omega\left(\omega\theta\sigma + 1\right) \epsk,
\end{align}
which further implies 
\begin{align*}
P(z^*)&=\frac{\theta}{2} \delta_{k+1}^2 + \delta_{k+1} - \delta_k - \frac{\theta\delta_{k+1}z^*}{(k+1)} + \frac{\theta(z^*)^2}{2(k+1)^{2}} -\frac{z^*}{(k+1)} + \frac{z^*}{k}\nonumber\\
& \leq \omega\left(\omega\theta\sigma + 1\right) \epsk- \frac{\theta\delta_{k+1}z^*}{(k+1)} + \frac{\theta(z^*)^2}{2(k+1)^{2}} -\frac{z^*}{(k+1)} + \frac{z^*}{k}. %
\end{align*}
Since $\epsk\leq \frac{\sigma}{k^{2}}$ and under the assumption that $\delta_{k+1} > \frac{C}{(k+1)}$, using the facts $(k+1)^{2}\leq 4k^{2}$ for all $k\geq 1$, we get
\begin{align*}
&\leq \frac{\omega \left(\omega \, \theta \, \sigma + 1\right) \sigma}{k^{2}} - \frac{\theta C}{4k^{2}}z^*
+ \frac{\theta}{2k^{2}}(z^*)^2 + \frac{1}{k^{2}}z^*\nonumber\\
&=\frac{Q(z^*)}{k^{2}},
\end{align*}
which, together with \eqref{Qz*} yields $P(z^*)\leq 0.$ This completes the proof.
\end{proof}

\begin{lemma}[Lemma 4.2 in~\citet{liu2019nonergodic}]
\label{prop:1}
Suppose the nonnegative sequence $\left\{\delta_k\right\}$ satisfies
\begin{eqnarray}\label{eq:ineqnonoise2}
\frac{E}{2} \delta_{k+1}^2 + \delta_{k+1} \leq \delta_k,~k=1,2,\ldots,
\end{eqnarray}where $E>0$ is a constant.
Then, we have
\begin{eqnarray}\label{eq:complexity1}
\delta_{k} \leq \frac{\max\left\{\delta_1,\frac{4}{E}\right\}}{k},~k=1,2,\ldots.
\end{eqnarray}
\end{lemma}
\begin{proof}
{Again we prove this by induction.} Clearly, the inequality \eqref{eq:complexity1} is true for $k=1$. Next, assuming \eqref{eq:complexity1} is true for some $k\geq 1$, we show it is also true for $k+1$. In fact, we have
\begin{align*}
\delta_{k+1} \leq \frac{-1+\sqrt{1+2E\delta_k}}{E} \leq &\  \frac{-1+\sqrt{1+2E\frac{\max\left\{\delta_1,\frac{4}{E}\right\}}{k}}}{E}\\=&\ \frac{2\max\left\{\delta_1,\frac{4}{E}\right\}}{k+\sqrt{k^2+2E\max\left\{\delta_1,\frac{4}{E}\right\}k}}\\
\leq&\  \frac{\max\left\{\delta_1,\frac{4}{E}\right\}}{k+1},
\end{align*}
where the first inequality is due to the inequality \eqref{eq:ineqnonoise2}, and the second inequality is due to the assumption that \eqref{eq:complexity1} holds for $k$.
\end{proof}

\begin{lemma}[Chapter 3 in~\citet{bertsekas2014constrained}]\label{prop:aug_lag_eq_and_ineq_same}
For $\lambda \geq 0$,
\begin{align}
    \min_{x \in \cX, s \in \R} \tilde{\cL}_\beta(x, s, \lambda) 
    &:= f(x) + \lambda \, [\dpd{a, x} - b + s^2] + \frac{\beta}{2} \, [\dpd{a, x} - b + s^2]^2 \label{eq:min_x_s_bar_L}\\
    \iff  
    \min_{x \in \cX} \cL^\dagger_\beta(x, \lambda) &:= f(x) + \frac{\beta}{2} \, \parens*{\bracks*{\max\parens*{\dpd{a, x} - b + \frac{\lambda}{\beta}, 0}}^2  - \frac{\lambda^2}{\beta^2}} \label{eq:min_x_L_dagger}.
\end{align}
As a result, $(\tilde{x}(\lambda), s(\lambda))$ is a solution of~\cref{eq:min_x_s_bar_L} if and only if $\tilde{x}(\lambda)$ is a solution to~\cref{eq:min_x_L_dagger} where
\begin{align}
\tilde{x}(\lambda) &:= \argmin_{x \in \cX} \cL^\dagger_\beta(x, \lambda),  \\ 
s(\lambda)^2  &= \max\parens*{- \frac{\lambda}{\beta} + \dpd{a, \tilde{x}(\lambda)} -b, 0}.
\end{align}
\end{lemma}
\begin{proof}
For a fixed $\lambda \geq 0$ and $x \in \cX$, we minimize $\bar{\cL}_\beta(x, s, \lambda)$ with respect to $s$,
\begin{align*}
\min_{s \in \R} \bar{\cL}_\beta(x, s, \lambda) &= \min_{s \in \R} \braces*{f(x) + \lambda \, [\dpd{a, x} - b + s^2] + \frac{\beta}{2} \, [\dpd{a, x} - b + s^2]^2} \tag{By the definition of $\bar{\cL}_\beta$}\\
&= \min_{z \geq 0} \braces*{\underbrace{f(x) + \lambda \, [\dpd{a, x} - b + z] + \frac{\beta}{2} \, [\dpd{a, x} - b + z]^2}_{:= g(z)}} \tag{Let $z = s^2$} \\
\intertext{Since $g$ is convex, we can take its derivative and find the global minimum,}
\implies (s^*)^2 = z^* &= \max\parens*{0, -\frac{\lambda}{\beta} - \dpd{a, x} + b}\tag{Since $z \geq 0$} \\
\end{align*}
Since $s^*$ is the optimal slack variable for an arbitrary $\lambda$ and $x$,
\begin{align*}
   &\min_{s \in \R} \bar{\cL}_\beta(x, s, \lambda) = \bar{\cL}_\beta(x, s^*, \lambda) \numberthis \label{eq:aug_lag_slack_algebra}\\
   &= f(x) + \lambda \, \bracks*{\dpd{a, x} - b + \max\parens*{0, -\frac{\lambda}{\beta} - \dpd{a, x} + b}} + \frac{\beta}{2} \, \bracks*{\dpd{a, x} - b + \max\parens*{0, -\frac{\lambda}{\beta} - \dpd{a, x} + b}}^2 \tag{By the definition of $\bar{\cL}_\beta$}\\
   &= f(x) + \lambda \, \bracks*{\max\parens*{\dpd{a, x} - b, -\frac{\lambda}{\beta}}} + \frac{\beta}{2} \, \bracks*{\max\parens*{\dpd{a, x} - b, -\frac{\lambda}{\beta}}}^2 \\
   &= f(x) + \lambda \, \bracks*{\max\parens*{\dpd{a, x} - b + \frac{\lambda}{\beta}, 0} - \frac{\lambda}{\beta}} + \frac{\beta}{2} \, \bracks*{\max\parens*{\dpd{a, x} - b + \frac{\lambda}{\beta}, 0} - \frac{\lambda}{\beta}}^2 \tag{Add/Subtract $\frac{\lambda}{\beta}$}\\
   &= f(x) + \frac{\beta}{2} \, \bracks*{\max\parens*{\dpd{a, x} - b + \frac{\lambda}{\beta}, 0} - \frac{\lambda}{\beta}}^2 + \lambda \, \max\parens*{\dpd{a, x} - b + \frac{\lambda}{\beta}, 0} - \frac{\lambda^2}{\beta} \\
   &= f(x) + \frac{\beta}{2} \, \parens*{\bracks*{\max\parens*{\dpd{a, x} - b + \frac{\lambda}{\beta}, 0} - \frac{\lambda}{\beta}}^2 + \frac{2 \, \lambda}{\beta} \, \max\parens*{\dpd{a, x} - b + \frac{\lambda}{\beta}, 0} - \frac{\lambda^2}{\beta^2}} \\
   &= f(x) + \frac{\beta}{2} \, \parens*{\bracks*{\max\parens*{\dpd{a, x} - b + \frac{\lambda}{\beta}, 0}}^2  - \frac{\lambda^2}{\beta^2}} \\
   &= \cL^\dagger_\beta(x, \lambda) \tag{By the definition of $\cL^\dagger_\beta$}
\end{align*}
Since $x \in \cX$, was arbitrary, we have
\begin{equation}
   \min_{x \in \cX, s \in \R} \bar{\cL}_\beta(x, s, \lambda)  = \min_{x \in \cX} \cL^\dagger_\beta(x, \lambda)
\end{equation}
\end{proof}


\begin{lemma}\label{lemma:aug_lag_subproblem_same}
For a given $\eps > 0$ and $\lambda \geq 0$, $x' \in \cX$ is a solution to
\begin{align}
    \cL^\dagger_\beta(x', \lambda) - \min_{x \in \cX}\cL^\dagger_\beta(x, \lambda) &\leq \eps
\end{align}
if and only if
\begin{align}
    \tilde{\cL}_\beta(x', s(x'), \lambda) - \min_{x \in \cX, s \in \R}\tilde{\cL}_\beta(x, s, \lambda) \leq \eps
\end{align}
where $s(x') = \max\parens*{0, - \frac{\lambda}{\beta} - \dpd{a, x'} + b}$.
\end{lemma}
\begin{proof}
It is sufficient to show that $\cL^\dagger_\beta(x', \lambda) = \tilde{\cL}_\beta(x', s(x'), \lambda)$
\begin{align*}
&= \Ls^\dagger_\beta(x', \lambda) = f(x') + \frac{\beta}{2} \, \parens*{\bracks*{\max\parens*{\dpd{a, x'} - b + \frac{\lambda}{\beta}, 0}}^2  - \frac{\lambda^2}{\beta^2}} \tag{By the definition of $\cL^\dagger_\beta$}\\
&= f(x') + \lambda \, \bracks*{\dpd{a, x'} - b + \underbrace{\max\parens*{0, -\frac{\lambda}{\beta} - \dpd{a, x'} + b}}_{:= s(x')}} +  \frac{\beta}{2} \, \bracks*{\dpd{a, x'} - b + \underbrace{\max\parens*{0, -\frac{\lambda}{\beta} - \dpd{a, x'} + b}}_{:=s(x')}}^2 \tag{Following~\cref{eq:aug_lag_slack_algebra}} \\
&= \tilde{\Ls}_\beta(x', s(x'), \lambda) \tag{By the definition of $\tilde{\cL}_\beta$}
\end{align*}
Combining with~\cref{prop:aug_lag_eq_and_ineq_same} finishes the proof.
\end{proof}





\begin{lemma}[Theorem 1 in~\citet{li2025smoothness}]\label{lemma:alm_dual_smooth}
Assuming $f$ is closed proper convex, the augmented Lagrangian dual function $d$ with penalty parameter $\beta > 0$ is $\frac{1}{\beta}$-smooth.
\end{lemma}
